# Supplementary material for: Slantwise convection and heat transport in icy moon oceans
Source: arXiv:2508.06480 ancillary file (2025-12-12)
Supplement: Supplementary file 1 [file SI_Slantwise_Convection.pdf]

# Supporting Information for "Slantwise convection and heat transport in the icy moon oceans"

Yaoxuan Zeng[1]and Malte F. Jansen[1]

[1]Department of the Geophysical Sciences, The University of Chicago, Chicago, IL 60637, USA

## Contents of this file

1. Text S1 to S3
2. Figures S1 to S5
3. Tables S1 to S2

Corresponding author: Yaoxuan Zeng (yxzeng@uchicago.edu)

**Text S1. Numerical details.** We set the parameters of our numerical simulations based on typical values for icy moon oceans. The buoyancy flux is calculated as $B = (Qg\alpha_T)/(\rho_0 c_p)$, where we use $\rho_0 = 10^3$ kg m$^{-3}$ for reference density and $c_p = 4000$ J kg$^{-1}$ K$^{-1}$ for the specific heat capacity of water. The bottom heat flux $Q$, gravitational acceleration $g$, and thermal expansivity $\alpha_T$ for various icy moons are listed in Table S1; in our simulations, we adopt $g = 0.1$ m s$^{-2}$ and $\alpha_T = 4 \times 10^{-5}$ K$^{-1}$, and vary $Q$ between 10 and 640 mW m$^{-2}$. A summary of the numerical simulation parameters is provided in Table 1. All simulations use uniform grid spacing in the zonal, meridional, and vertical directions.

We focus on the ocean interior, where the horizontally and temporally averaged temperature profile is approximately linear. To identify the boundaries between the interior and the thermal boundary layers, we perform a linear fit to the temperature profile, starting from the domain center and extending outward toward both the top and bottom. The fit is carried out incrementally over increasing depth and is terminated when the coefficient of determination falls below $r^2 = 0.998$. From this fit, we obtain the depth of the interior, $H$, and the corresponding buoyancy gradient, $|\nabla b|$, as illustrated in Fig. 1b.

In our simulations, subgrid-scale eddies are not explicitly resolved but are parameterized using the Smagorinsky closure, in which viscosity and diffusivity are determined by local velocity gradients, grid spacing, and prescribed coefficients $A_{\nu,\mathrm{smag}}$ and $A_{\kappa,\mathrm{smag}}$ (Smagorinsky, 1963; Smagorinsky et al., 1993):

$$\nu_{smag} = 2\sqrt{2}A_{\nu,smag}V_{grid}^{2/3}\sqrt{v_{xx}^2 + v_{yy}^2 + v_{RR}^2 + \frac{(v_{xy}+v_{yx})^2}{2} + \frac{(v_{xR}+v_{Rx})^2}{2} + \frac{(v_{Ry}+v_{yR})^2}{2}}, \tag{1}$$

$$\kappa_{smag} = 2\sqrt{2}A_{\kappa,smag}V_{grid}^{2/3}\sqrt{v_{xx}^2 + v_{yy}^2 + v_{RR}^2 + \frac{(v_{xy}+v_{yx})^2}{2} + \frac{(v_{xR}+v_{Rx})^2}{2} + \frac{(v_{Ry}+v_{yR})^2}{2}}, \tag{2}$$

where $V_{grid}$ is the grid volume, and $v_{ij} \equiv \partial v_i/\partial j$, $i, j = x, y, R$ are the velocity gradients. Values of $A_{\nu,\mathrm{smag}}$ are listed in Table 1 and we set $A_{\kappa,\mathrm{smag}} = 0.1A_{\nu,\mathrm{smag}}$ in our simulations.

For comparison with previous direct numerical simulations that characterize planetary parameters using the Rayleigh number $\mathrm{Ra} = \Delta b_{\mathrm{domain}} H_{\mathrm{domain}}^3/(\nu\kappa)$ and the Ekman number $\mathrm{Ek} = \nu/(\Omega H_{\mathrm{domain}}^2)$, we estimate Ra and Ek based on the diagnosed horizontally averaged buoyancy contrast between the two plates and the domain-averaged Smagorinsky eddy viscosity and diffusivity from a single snapshot. Here, both $\Delta b_{\mathrm{domain}}$ and $H_{\mathrm{domain}}$ are evaluated across the full domain, differing from the ocean interior definition used in the main text, to ensure consistency with previous studies. The transition to the non-rotating regime is given by $\mathrm{Ra}_{\mathrm{T,NR}} = 100\mathrm{Ek}^{-12/7}$, and the transition to the rapidly rotating regime is given by $\mathrm{Ra}_{\mathrm{T,RR}} = 0.4\mathrm{Ek}^{-8/5}$, following Gastine, Wicht, and Aubert (2016). The resulting values place our simulations in the transitional regime, $\mathrm{Ra}_{\mathrm{T,RR}} < \mathrm{Ra} < \mathrm{Ra}_{\mathrm{T,NR}}$, consistent with that expected for icy moon oceans (Table S2).

To assess the sensitivity to the sub-grid eddy parameterization, we conducted one simulation with viscosity and diffusivity parameters, $A_{\kappa,smag}$ and $A_{\nu,smag}$, reduced by a factor of 10 ($L60_{\mathrm{lowvisc}}$), and another low-resolution simulation with grid spacing doubled

($L60_{\mathrm{lowres}}$), both compared to the control simulation $L60_{\mathrm{Ctrl}}$. In the low-viscosity case, results changed by less than 3%, indicating that viscosity and diffusivity have minimal influence on interior ocean dynamics under our simulation parameters. In the low-resolution case, the buoyancy gradient and the meridional heat flux show very little change (less than 2%), while the interior depth decreased by about 10%. This suggests that the coarser resolution thickens the boundary layers, likely due to increased effective viscosity and diffusivity from the larger grid spacing, but does not significantly affect the interior dynamics.

We also use a free surface as the top boundary condition in our simulations. To assess its impact, we performed an additional simulation with a rigid lid at the top ($L60_{\mathrm{RigidLid}}$), comparing it to the corresponding simulation with a free surface ($L60_{0.5L_y}$). The results only differed by 1%, indicating that the top boundary condition has little effect on heat transport. This insensitivity arises because the barotropic deformation radius, $L_D = \sqrt{gH}/(2\Omega)$, is much larger than the domain scale in all simulations, with $L_D/L_{\mathrm{domain}}$ ranging from 40 to 500. As a result, variations in surface elevation have negligible dynamical influence.

**Text S2. Eddy scale of the heat transport.** As shown in Section 3, the axial ($\mathbf{e_z}$) and the radial ($\mathbf{e_r}$) heat fluxes are of comparable magnitude. To guide the development of parameterizations, which are intended to represent the effects of unresolved subgrid-scale dynamics, it is important to assess whether the processes responsible for these transports occur at different spatial scales. If a clear scale separation exists, it may be possible to

explicitly resolve the larger-scale process in global simulations while parameterizing the smaller-scale one.

We estimate the characteristic length scales of heat transport by computing the spectral centroids $(k_x^c, k_y^c)$ of the axial and radial heat transport cross-spectra in the ocean interior. These spectra are defined by $\mathrm{Re}(\hat{v}_z\hat{T}^*)$ for axial transport and $\mathrm{Re}(\hat{v}_r\hat{T}^*)$ for radial transport, where the hat denotes the Fourier transform and the asterisk denotes the complex conjugate. The spectral centroids are given by:

$$k_x^c = \left(\frac{\iint k_x^2|\hat{P}|dk_x dk_y}{\iint |\hat{P}|dk_x dk_y}\right)^{1/2}, \; k_y^c = \left(\frac{\iint k_y^2|\hat{P}|dk_x dk_y}{\iint |\hat{P}|dk_x dk_y}\right)^{1/2}, \tag{3}$$

where $\hat{P}$ represents the cross-spectrum of either $\mathrm{Re}(\hat{v}_r\hat{T}^*)$ or $\mathrm{Re}(\hat{v}_z\hat{T}^*)$.

We find that the eddy length scales associated with heat transport in the axial and radial directions are of comparable magnitude, indicating no clear scale separation between them (Fig. S1). In the polar simulation ($\theta = 90°$), strong cancellation between positive and negative contributions to the radial heat transport results in a negligible net radial flux (Table 2).

The radial heat transport spectrum (first row in Fig. S1) exhibits a dip in energy near $k_x = 0$, indicating that the zonally symmetric mode primarily transports heat along the rotation axis. This result is consistent with the linear instability analyses of Flasar and Gierasch (1978) and Hathaway, Gilman, and Toomre (1979), which showed that the most unstable symmetric modes correspond to slantwise convection and preferentially transport heat along the rotation axis.

More generally, the heat transport spectrum is nearly isotropic near the pole and becomes increasingly anisotropic toward lower latitudes. There is some anisotropy present in the $\theta = 90°$ simulation, which arises from the domain geometry, where the zonal extent is shorter than the meridional one. At lower latitudes, eddies become elongated in the meridional direction (i.e., shifted toward smaller $k_y$), as also evident in the snapshots (Fig. 2). This anisotropy is consistent with the findings of Currie, Barker, Lithwick, and Browning (2020) and likely results from the geometric projection of slantwise convection onto the horizontal plane: at the pole, where the rotation axis is vertical, the projection is isotropic; at lower latitudes, the rotation axis tilts in the meridional direction, introducing anisotropy and leading to meridional elongation.

**Text S3. Effects of zonal jets.** Previous studies have shown that zonal jets can influence convective heat transport. Novi, von Hardenberg, Hughes, Provenzale, and Spiegel (2019) and Currie et al. (2020) found that vertical heat transport along gravity increases with latitude in the presence of zonal jets. Currie et al. (2020) further demonstrated that when the zonal domain is longer than the meridional domain, meridional jets form instead of zonal ones. In such cases, vertical heat transport increases with latitude up to approximately 60°, and remains nearly constant higher than 60° (see their Fig. 4).

In our simulations, zonal jets are present, and the vertical heat transport (i.e., along the direction of gravity) increases with latitude, consistent with earlier findings. To investigate the influence of jets, we conducted sensitivity tests by modifying the horizontal domain aspect ratio and introducing linear bottom drag. At $\theta = 60°$, we tested three aspect ratios:

$L_x : L_y = 7 : 15$ ($L60_{\mathrm{Ctrl}}$), $14 : 15$ ($L60_{0.5L_y}$), and $28 : 15$ ($L60_{2L_x 0.5L_y}$). Additionally, we performed a simulation with linear bottom drag ($L60_{\mathrm{drag}}$), in which bottom-layer velocities were relaxed to zero at a rate of $2.5 \times 10^{-4}$ s$^{-1}$, which suppresses jet formation.

In simulations $L60_{0.5L_y}$ and $L60_{\mathrm{Ctrl}}$, zonal jets develop (Fig. S5a & b). Although their jet magnitudes differ by a factor of two, the resulting buoyancy gradient and flux vary by less than 4% (Table 2), suggesting that jet strength has a limited impact on heat transport. In $L60_{2L_x 0.5L_y}$, where the zonal domain is wider than the meridional one, meridional jets form instead (Fig. S5c), consistent with Currie et al. (2020). In this case, the meridional heat flux reverses sign ($B_y = B_z \cos\theta - B_r \sin\theta < 0$; Table 2). However, as discussed in Section 5, the $\beta$ effect in real icy moon oceans is expected to inhibit the formation of meridional jets (Rhines, 1975; Vallis, 2017), making such a scenario unlikely to occur in real oceans. In $L60_{\mathrm{drag}}$, linear drag suppresses jet formation, and domain-scale eddies dominate (Fig. S5d), reducing the meridional heat flux $B_y$ by a factor of 5, although it remains poleward.

These results suggest that the presence and orientation of jets significantly affect meridional heat transport. Across all four simulations, however, the vertical buoyancy flux remains close to the imposed value, and buoyancy gradients vary by less than 10%, indicating that vertical transport at $\theta = 60°$ is less sensitive to jet configuration. Notably, in the other two outlier cases in Fig. 3b ($L15_{\mathrm{Ctrl}}$ and $L15_{0.625\Omega}$), jets exhibit strong meandering (Fig. S5e & f), in contrast to the relatively straight jets in other simulations. This also suggests that the structure of the zonal jets may influence convective heat transport. Quantifying this effect is left for future work.

## References

Aurnou, J. M., Horn, S., & Julien, K. (2020). Connections between nonrotating, slowly rotating, and rapidly rotating turbulent convection transport scalings. *Physical Review Research*, *2*(4), 043115.

Currie, L. K., Barker, A. J., Lithwick, Y., & Browning, M. K. (2020). Convection with misaligned gravity and rotation: simulations and rotating mixing length theory. *Monthly Notices of the Royal Astronomical Society*, *493*(4), 5233–5256.

Flasar, F. M., & Gierasch, P. J. (1978). Turbulent convection within rapidly rotating superadiabatic fluids with horizontal temperature gradients. *Geophysical & Astrophysical Fluid Dynamics*, *10*(1), 175–212.

Gastine, T., Wicht, J., & Aubert, J. (2016). Scaling regimes in spherical shell rotating convection. *Journal of Fluid Mechanics*, *808*, 690–732.

Hathaway, D. H., Gilman, P. A., & Toomre, J. (1979). Convective instability when the temperature gradient and rotation vector are oblique to gravity. i. fluids without diffusion. *Geophysical & Astrophysical Fluid Dynamics*, *13*(1), 289–316.

Novi, L., von Hardenberg, J., Hughes, D. W., Provenzale, A., & Spiegel, E. A. (2019). Rapidly rotating rayleigh-bénard convection with a tilted axis. *Physical Review E*, *99*(5), 053116.

Rhines, P. B. (1975). Waves and turbulence on a beta-plane. *Journal of Fluid Mechanics*, *69*(3), 417–443.

Smagorinsky, J. (1963). General circulation experiments with the primitive equations: I. the basic experiment. *Monthly weather review*, *91*(3), 99–164.

Smagorinsky, J., Galperin, B., & Orszag, S. (1993). Large eddy simulation of complex engineering and geophysical flows. *Evolution of physical oceanography*, 3–36.

Soderlund, K. M. (2019). Ocean dynamics of outer solar system satellites. *Geophysical Research Letters*, *46*(15), 8700–8710.

Vallis, G. K. (2017). *Atmospheric and oceanic fluid dynamics.* Cambridge University Press.

Zeng, Y., & Jansen, M. F. (2021). Ocean circulation on enceladus with a high-versus low-salinity ocean. *The Planetary Science Journal*, *2*(4), 151.

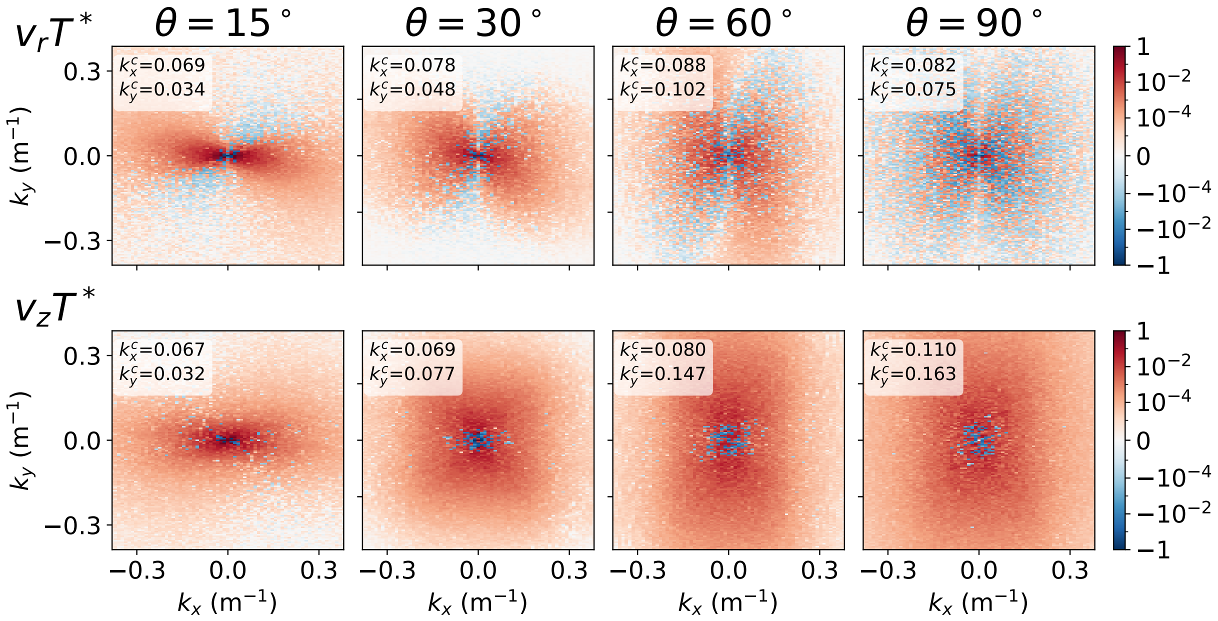


**Figure S1. Horizontal cross-spectra of the eddy heat transport.** From left to right, the columns show results from the control simulations at different latitudes: $L15_{\mathrm{Ctrl}}$, $L30_{\mathrm{Ctrl}}$, $L60_{\mathrm{Ctrl}}$, and $L90_{\mathrm{Ctrl}}$. The upper and lower rows show the cross-spectra for radial and axial heat transport, $\mathrm{Re}(\hat{v}_r\hat{T}^*)$ and $\mathrm{Re}(\hat{v}_z\hat{T}^*)$, respectively. Spectra are computed from averages of horizontal slices within the interior region using a single snapshot. Spectral centroids are indicated in the upper-left corner of each panel.

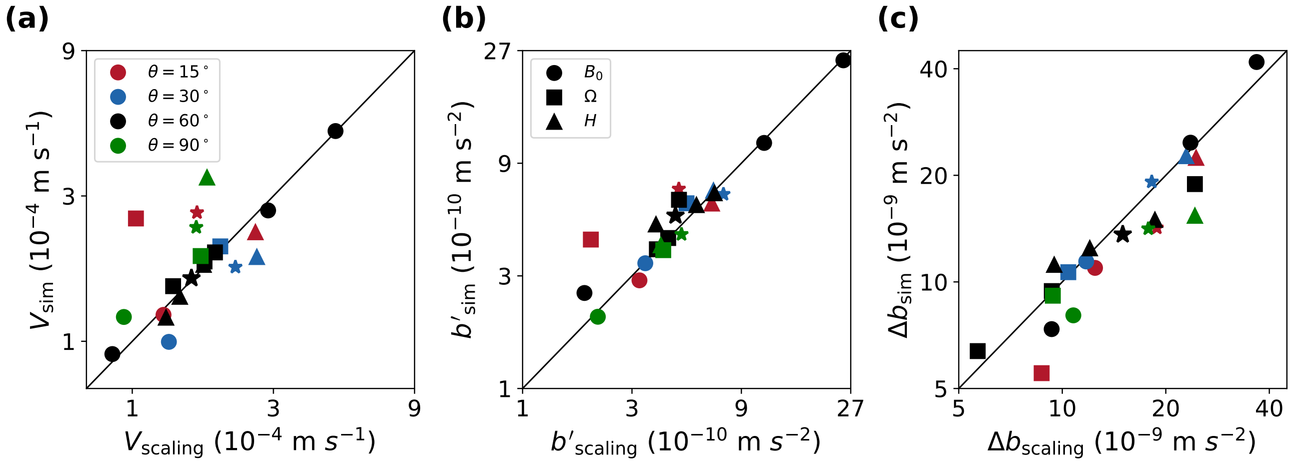


**Figure S2. The CIA scaling compared with simulation results.** (a)–(c) show the CIA scalings for the eddy velocity, $V = v_r'^2 + v_z'^2$, buoyancy perturbation $b'$, and buoyancy contrast $\Delta b$, respectively, where primes denote deviations from the horizontal average. The vertical axis shows simulation results, while the horizontal axis shows the corresponding theoretical CIA scalings: $V \sim \Delta b(2\Omega)^{-1}$, $b' \sim \Delta b^{3/2}(2\Omega)^{-1}H^{-1/2}$, and $\Delta b \sim B^{2/5}(2\Omega)^{4/5}H^{1/5}$ (c.f. Aurnou et al. (2020) and references therein). All scalings are evaluated from a single snapshot and averaged over the interior region. Note that $B$ denotes the magnitude of the total buoyancy flux, $B = (B_r^2 + B_z^2)^{1/2}$, rather than the individual components $B_r$ and $B_z$, which are discussed in Section 3. Pre-factors are fitted using simulations at $\theta = 60°$ and applied uniformly across all cases: 1.16 in (a), 0.86 in (b), and 0.51 in (c). Symbols are consistent with those in Fig. 3.

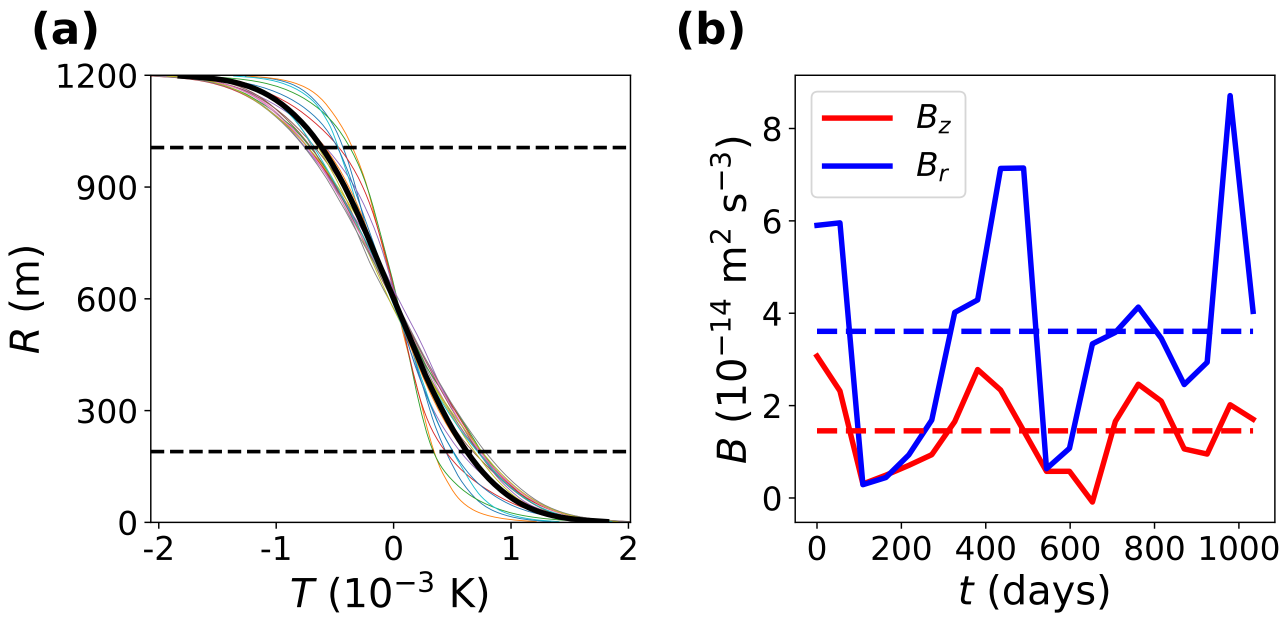


**Figure S3. Time series of the temperature profile and buoyancy flux in simulation** $L15_{0.625\Omega}$. (a) Horizontally averaged temperature profiles. Thin lines show individual snapshots, and the thick black line shows the time-averaged profile. Black dashed lines mark the boundaries between the interior and the boundary layers. (b) Time series of buoyancy flux in the axial ($B_z$, red) and radial ($B_r$, blue) directions. Solid lines show the time series, while dashed lines indicate the corresponding time averages.

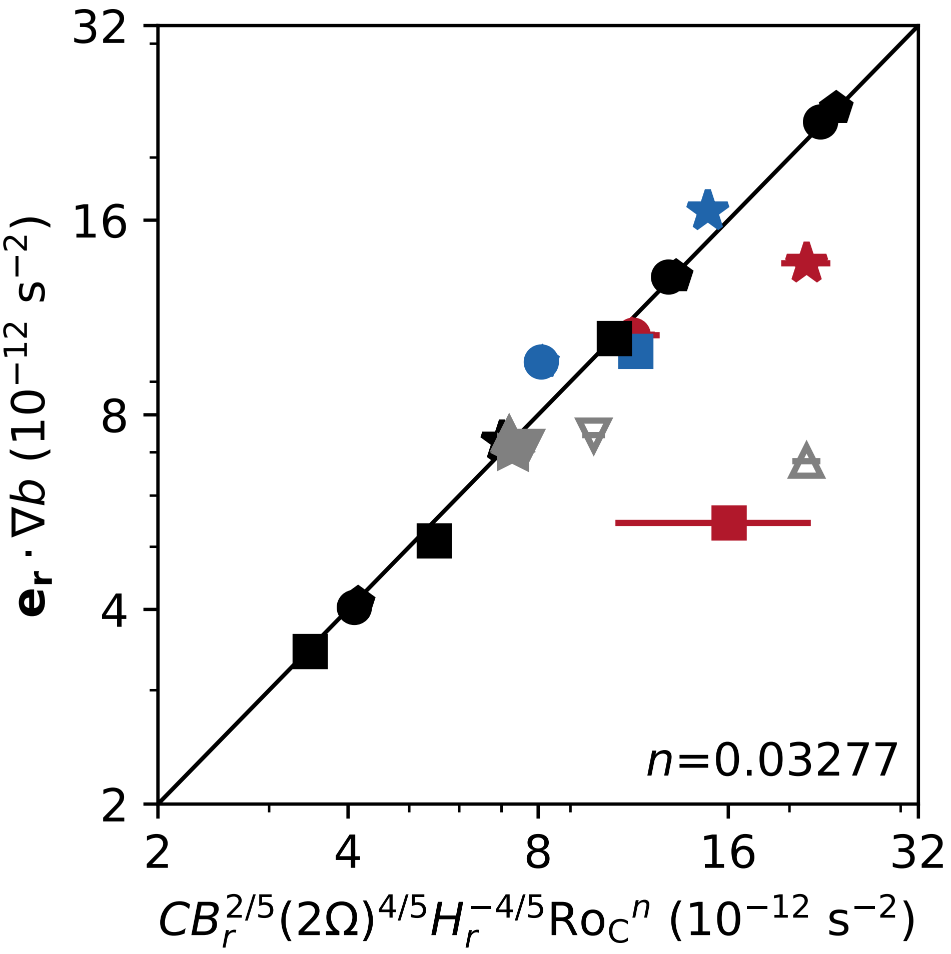


**Figure S4. Scaling of the radial ($\mathbf{e_r}$) flux-gradient relation with best-fit exponents.** According to the Buckingham $\pi$ theorem, there is one non-dimensional parameter that governs the buoyancy flux–gradient relation. We define it as $\mathrm{Ro_C} = |B_r|^{1/2}(2\Omega)^{-3/2}H_r^{-1}$, motivated by the convective Rossby number but using the interior depth projected in the radial direction, $H_r$, as the characteristic length scale. We assume a flux–gradient relation of the form $\mathbf{e_r} \cdot \nabla b = CB_r^{2/5}(2\Omega)^{4/5}H_r^{-4/5}\mathrm{Ro_C}^n$, and fit the pre-factor $C$ and exponent $n$ using simulations at $\theta = 60°$, then apply the fit across all latitudes. Symbols match those in Fig. 3. The fitted exponent $n$ is close to zero, supporting the use of the semi-empirical scaling (Equation 7).

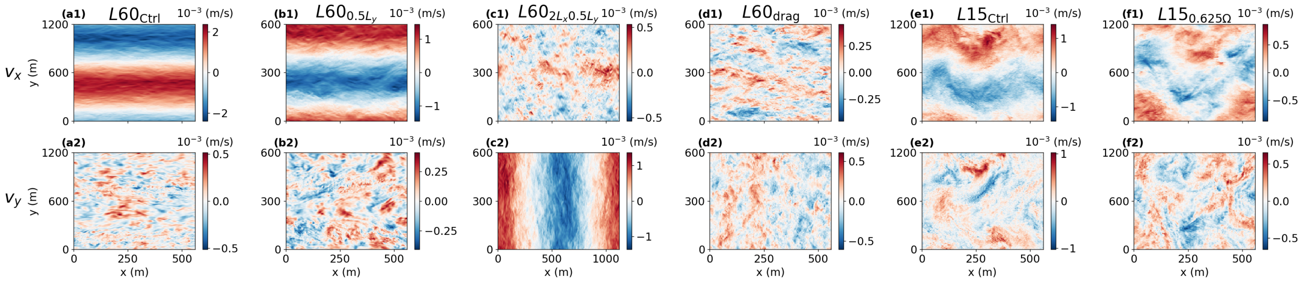


**Figure S5. Horizontal snapshots of the horizontal velocity fields at mid-depth ($R = 600$ m).** The first and second rows show the zonal velocity $v_x$ and the meridional velocity $v_y$, respectively. (a)–(c) show simulations with varying horizontal aspect ratios: $L60_{\mathrm{Ctrl}}$, $L60_{0.5L_y}$, and $L60_{2L_x 0.5L_y}$. (d) shows the simulation with linear bottom drag applied to suppress jet formation ($L60_{\mathrm{drag}}$). (e) and (f) show simulations $L15_{\mathrm{Ctrl}}$ and $L15_{0.625\Omega}$. In all other simulations, relatively strong and straight jets form, resembling those in $L60_{0.5L_y}$ and $L60_{\mathrm{Ctrl}}$.

**Table S1.** Icy moon ocean parameters. The first section is adapted from Table 1 in Soderlund (2019). Estimates involving negative thermal expansivity are excluded, as such values suppress convection driven by bottom heating (Zeng & Jansen, 2021). The second section presents derived quantities based on these parameters.

| Parameter | Enceladus | Titan | Europa | Ganymede |
| --- | --- | --- | --- | --- |
| $Q$ (mW m$^{-2}$) | 16–83 | 14–20 | 23–123 | 15–107 |
| $g$ (m s$^{-2}$) | 0.1 | 1.4 | 1.3 | 1.4 |
| $\alpha_T$ ($10^{-4}$K$^{-1}$) | 0.1–1.3 | 0.4–4.2 | 1.9–2.5 | 1.9–4.4 |
| $2\Omega$ (s$^{-1}$) | $1.1 \times 10^{-4}$ | $9.2 \times 10^{-6}$ | $4.2 \times 10^{-5}$ | $2.0 \times 10^{-5}$ |
| $H$ ($10^3$ km) | 11–63 | 91–420 | 97–131 | 24–518 |
| $B$ ($10^{-14}$ m$^2$ s$^{-3}$) | 0.4–27.0 | 19.6–294 | 148–938 | 120–1650 |
| $l_{\mathrm{plume}}$ ($^\circ$) | 0.006–0.039 | 0.027–0.113 | 0.024–0.044 | 0.026–0.106 |

**Table S2.** Ekman and Rayleigh numbers for numerical simulations. See Supplementary Text S1 for details.

| Name | Ek | Ra | $\mathrm{Ra}_{\mathrm{T,RR}} = 0.4\mathrm{Ek}^{-8/5}$ | $\mathrm{Ra}_{\mathrm{T,NR}} = 100\mathrm{Ek}^{-12/7}$ |
|---|---|---|---|---|
| $L60_{\mathrm{Ctrl}}$ | $7.91 \times 10^{-8}$ | $4.96 \times 10^{12}$ | $9.22 \times 10^{10}$ | $1.49 \times 10^{14}$ |
| $L60_{0.25B}$ | $4.81 \times 10^{-8}$ | $8.42 \times 10^{12}$ | $2.05 \times 10^{11}$ | $3.51 \times 10^{14}$ |
| $L60_{4B}$ | $1.21 \times 10^{-7}$ | $3.48 \times 10^{12}$ | $4.66 \times 10^{10}$ | $7.20 \times 10^{13}$ |
| $L60_{16B}$ | $2.08 \times 10^{-7}$ | $2.00 \times 10^{12}$ | $1.96 \times 10^{10}$ | $2.84 \times 10^{13}$ |
| $L60_{0.39\Omega}$ | $2.12 \times 10^{-7}$ | $1.95 \times 10^{12}$ | $1.90 \times 10^{10}$ | $2.75 \times 10^{13}$ |
| $L60_{0.625\Omega}$ | $1.34 \times 10^{-7}$ | $2.85 \times 10^{12}$ | $3.97 \times 10^{10}$ | $6.06 \times 10^{13}$ |
| $L60_{1.6\Omega}$ | $4.91 \times 10^{-8}$ | $8.01 \times 10^{12}$ | $1.98 \times 10^{11}$ | $3.38 \times 10^{14}$ |
| $L60_{0.25H}$ | $2.13 \times 10^{-7}$ | $1.96 \times 10^{12}$ | $1.90 \times 10^{10}$ | $2.75 \times 10^{13}$ |
| $L60_{0.5H}$ | $1.27 \times 10^{-7}$ | $3.18 \times 10^{12}$ | $4.34 \times 10^{10}$ | $6.66 \times 10^{13}$ |
| $L60_{2H}$ | $4.71 \times 10^{-8}$ | $8.78 \times 10^{12}$ | $2.12 \times 10^{11}$ | $3.64 \times 10^{14}$ |
| $L15_{\mathrm{Ctrl}}$ | $1.48 \times 10^{-7}$ | $1.09 \times 10^{12}$ | $3.37 \times 10^{10}$ | $5.09 \times 10^{13}$ |
| $L15_{0.25B}$ | $5.14 \times 10^{-8}$ | $6.86 \times 10^{12}$ | $1.84 \times 10^{11}$ | $3.13 \times 10^{14}$ |
| $L15_{0.625\Omega}$ | $1.49 \times 10^{-7}$ | $1.39 \times 10^{12}$ | $3.34 \times 10^{10}$ | $5.03 \times 10^{13}$ |
| $L15_{2H}$ | $5.22 \times 10^{-8}$ | $6.67 \times 10^{12}$ | $1.79 \times 10^{11}$ | $3.04 \times 10^{14}$ |
| $L30_{\mathrm{Ctrl}}$ | $8.19 \times 10^{-8}$ | $5.14 \times 10^{12}$ | $8.73 \times 10^{10}$ | $1.41 \times 10^{14}$ |
| $L30_{0.25B}$ | $5.00 \times 10^{-8}$ | $8.76 \times 10^{12}$ | $1.92 \times 10^{11}$ | $3.28 \times 10^{14}$ |
| $L30_{0.625\Omega}$ | $1.34 \times 10^{-7}$ | $3.06 \times 10^{12}$ | $3.96 \times 10^{10}$ | $6.04 \times 10^{13}$ |
| $L30_{2H}$ | $4.93 \times 10^{-8}$ | $9.06 \times 10^{12}$ | $1.97 \times 10^{11}$ | $3.37 \times 10^{14}$ |
| $L90_{\mathrm{Ctrl}}$ | $8.18 \times 10^{-8}$ | $4.53 \times 10^{12}$ | $8.74 \times 10^{10}$ | $1.41 \times 10^{14}$ |
| $L90_{0.25B}$ | $4.92 \times 10^{-8}$ | $7.41 \times 10^{12}$ | $1.98 \times 10^{11}$ | $3.38 \times 10^{14}$ |
| $L90_{0.625\Omega}$ | $1.30 \times 10^{-7}$ | $3.01 \times 10^{12}$ | $4.17 \times 10^{10}$ | $6.39 \times 10^{13}$ |
| $L90_{2H}$ | $1.90 \times 10^{-7}$ | $1.03 \times 10^{12}$ | $2.27 \times 10^{10}$ | $3.33 \times 10^{13}$ |
| $L60_{\mathrm{lowvisc}}$ | $1.04 \times 10^{-8}$ | $2.86 \times 10^{14}$ | $2.37 \times 10^{12}$ | $4.83 \times 10^{15}$ |
| $L60_{\mathrm{lowres}}$ | $2.14 \times 10^{-7}$ | $7.22 \times 10^{11}$ | $1.88 \times 10^{10}$ | $2.72 \times 10^{13}$ |
| $L60_{\mathrm{RigidLid}}$ | $8.90 \times 10^{-8}$ | $3.77 \times 10^{12}$ | $7.64 \times 10^{10}$ | $1.22 \times 10^{14}$ |
| $L60_{\mathrm{drag}}$ | $8.98 \times 10^{-8}$ | $3.12 \times 10^{12}$ | $7.54 \times 10^{10}$ | $1.20 \times 10^{14}$ |
| $L60_{0.5L_y}$ | $8.24 \times 10^{-8}$ | $4.44 \times 10^{12}$ | $8.64 \times 10^{10}$ | $1.39 \times 10^{14}$ |
| $L60_{2L_x0.5L_y}$ | $8.50 \times 10^{-8}$ | $3.72 \times 10^{12}$ | $8.23 \times 10^{10}$ | $1.32 \times 10^{14}$ |
